# Supplementary material for: Cutting Polygons into Small Pieces with Chords: Laser-Based Localization
Source: arXiv:2006.15089 source file (2020-06-26)
Supplement: Supplementary file 1 [file appendix.tex]

\begin{table}[!htb]
	\centering
	\begin{tabular}{ |c|c|c|c|c|  }
		\hline
		\multicolumn{1}{|c|}{ } & \multicolumn{2}{|c|}{Convex cell restriction} & \multicolumn{2}{|c|}{No convex restriction} \\
		
		\hline
		& Primal & Dual & Primal & Dual\\
		\hline
		Area  & $O(\log r)$  & $O(r^{2})$ & $O(\log r)$ & $O(r^{2})$\\
		\hline
		Diameter & $O(1)$	 & $O(r)$ & bicriteria  & $O(r)$\\
		\hline
	\end{tabular}
	\label{tab:results}
	\caption{ Approximation bounds for variants of the problem. Here, $r$ is the number of reflex vertices in the polygon.}
\end{table}

\section{Problem Statement}
A polygonal region can be cut into multiple cell by laying out multiple lasers. The boundary of each sub division is made of either lasers completely or partly lasers and partly original boundary of the polygonal region itself. \\
\textbf{Definition:}
Diameter of a cell is defined as maximum Euclidean distance between any two points in that cell.\\
Let, after deploying lasers over the polygonal region, the induced cells are $s_{1}, s_{2},\ldots, s_{k}$ and their corresponding areas are $a_{1}, a_{2},\ldots ,a_{k}$ and diameters are $d_{1}, d_{2},\ldots,d_{k}$. \\

\subsection{Problem 1}
Given a simple convex polygon $P$ and a diameter budget $\delta$, find the smallest number of lasers such that each partition created by the cuts of lasers has diameter less than equal to $\delta$.

\subsection{Problem 2}
Given a simple polygon $P$ (may be non-convex) and a diameter budget $\delta$, find the smallest number of lasers such that polygon $P$ is cut into convex pieces and each convex partition created by the cuts of lasers has diameter less  than equal to $\delta$.

\subsection{Problem 3}
Given a simple convex polygon $P$ and $K$ lasers, position the lasers in $P$ such that $P$ is cut into convex pieces and maximum diameter of all the convex pieces is minimized.

\subsection{Problem 4}
This is dual of problem 3. Given a budget diameter $d$, find out minimum number of lasers such that maximum diameter of a induced cells is less than equal to budget $d$.

\subsection{Problem 5}
Given a simple convex polygon $P$ and a diameter budget $\delta$, find the smallest number of lasers such that each partition created by the cuts of lasers has diameter less  than equal to $\delta$.

\subsection{Problem 6}
Given a simple polygon $P$ (may be non-convex) and a diameter budget $\delta$, find the smallest number of lasers such that polygon $P$ is cut into convex pieces and each convex partition created by the cuts of lasers has diameter less  than equal to $\delta$.

\subsection{Problem 7}
Given a simple convex polygon $P$ and $K$ lasers, position the lasers in $P$ such that $P$ is cut into convex pieces and maximum diameter of all the convex pieces is minimized.

\subsection{Problem 8}
Given a simple polygon $P$ with $R$ reflex vertices and $K$ lasers, position the lasers in $P$ such that $P$ is cut into convex pieces and maximum diameter of all the convex pieces cut by the lasers is minimized.

\section{Decomposing into Convex Pieces}
We will first try to solve the problems with added constraint that each induced cell has to be convex.\\

\subsection{Problem 2 :} Given a simple polygon $P$ (may be non-convex) and a diameter budget $\delta$, find the smallest number of lasers such that polygon $P$ is cut into convex pieces and each convex partition created by the cuts of lasers has diameter less  than equal to $\delta$.

\subsubsection{Algorithm:}
\subsection{Problem 3 :} Given a simple convex polygon $P$ and $K$ lasers, position the lasers in $P$ such that $P$ is cut into convex pieces and maximum diameter of all the convex pieces is minimized.

\subsubsection{Algorithm}
 Divide $P$'s boundary into $\frac{K}{2}$ equal parts and put 2 lasers orthogonally from each point.

\subsubsection{Approximation Bound:}
\begin{theorem}
	Problem 3 can be solved by a  polynomial time $4\sqrt{2}\pi$ approximation algorithm.
\end{theorem}

\begin{proof}
	$K$ lasers can touch $2K$ points. So if we evenly distribute $2K$ points along the polygonal boundary, then the maximum length between any points will be minimized. This maximum length will be then $\frac{\per(P)}{2K}$.\\
	The minimum diameter possible with this length is $\frac{\per(P)}{2\pi K}$ as each piece is convex and circle is the optimum convex shape which minimize diameter given it's perimeter. Lets call the optimal diameter of polygon $P$ is $C^{*}$.
	
	\begin{equation}
	C^{*} \geq \frac{\per(P)}{2\pi K}
	\end{equation}
	
	As we divided $P$'s boundary into $\frac{K}{2}$ equal parts and put 2 lasers orthogonally from each point, so the length between any 2 points is less than equal to $\frac{2\,\per(P)}{K}$. \\
	Lets $C$ be the maximum diameter of all convex pieces.
	
	\begin{equation}
	\begin{aligned}
	C &\leq \sqrt{\Big(\frac{2\,\per(P)}{K}\Big)^{2} + \Big(\frac{2\,\per(P)}{K}\Big)^{2}} \\
	  &\leq 2\sqrt{2}\frac{\per(P)}{K} \\
	  &\leq 4\sqrt{2}\pi C^{*}
	  \end{aligned}
	\end{equation}
	
\end{proof}
Time Complexity : $O(\frac{\per(P)}{K})$ \\ \\

\subsection{Problem 4 :} Given a simple polygon $P$ with $R$ reflex vertices and $K$ lasers, position the lasers in $P$ such that $P$ is cut into convex pieces and maximum diameter of all the convex pieces cut by the lasers is minimized.

\subsubsection{Algorithm}
\begin{enumerate}
	\item Compute the convex hull of polygon $P$ and call it $\conv(P)$.
	\item Divide $\conv(P)$'s boundary into $\frac{\per(\conv(P))}{2K}$ equal parts and put 2 lasers orthogonally from each point.
	\item Now if a laser has passed out of polygonal region $m$ times, replace that laser with $m$ lasers such that each laser is fully contained in the polygonal region.
\end{enumerate}

\subsubsection{Approximation Bound:}
\begin{theorem}
	Problem 4 can be solved by a polynomial time $O(R)$ approximation algorithm.
\end{theorem}

\begin{figure*}[h]
	\centering
	\includegraphics[scale=0.5]{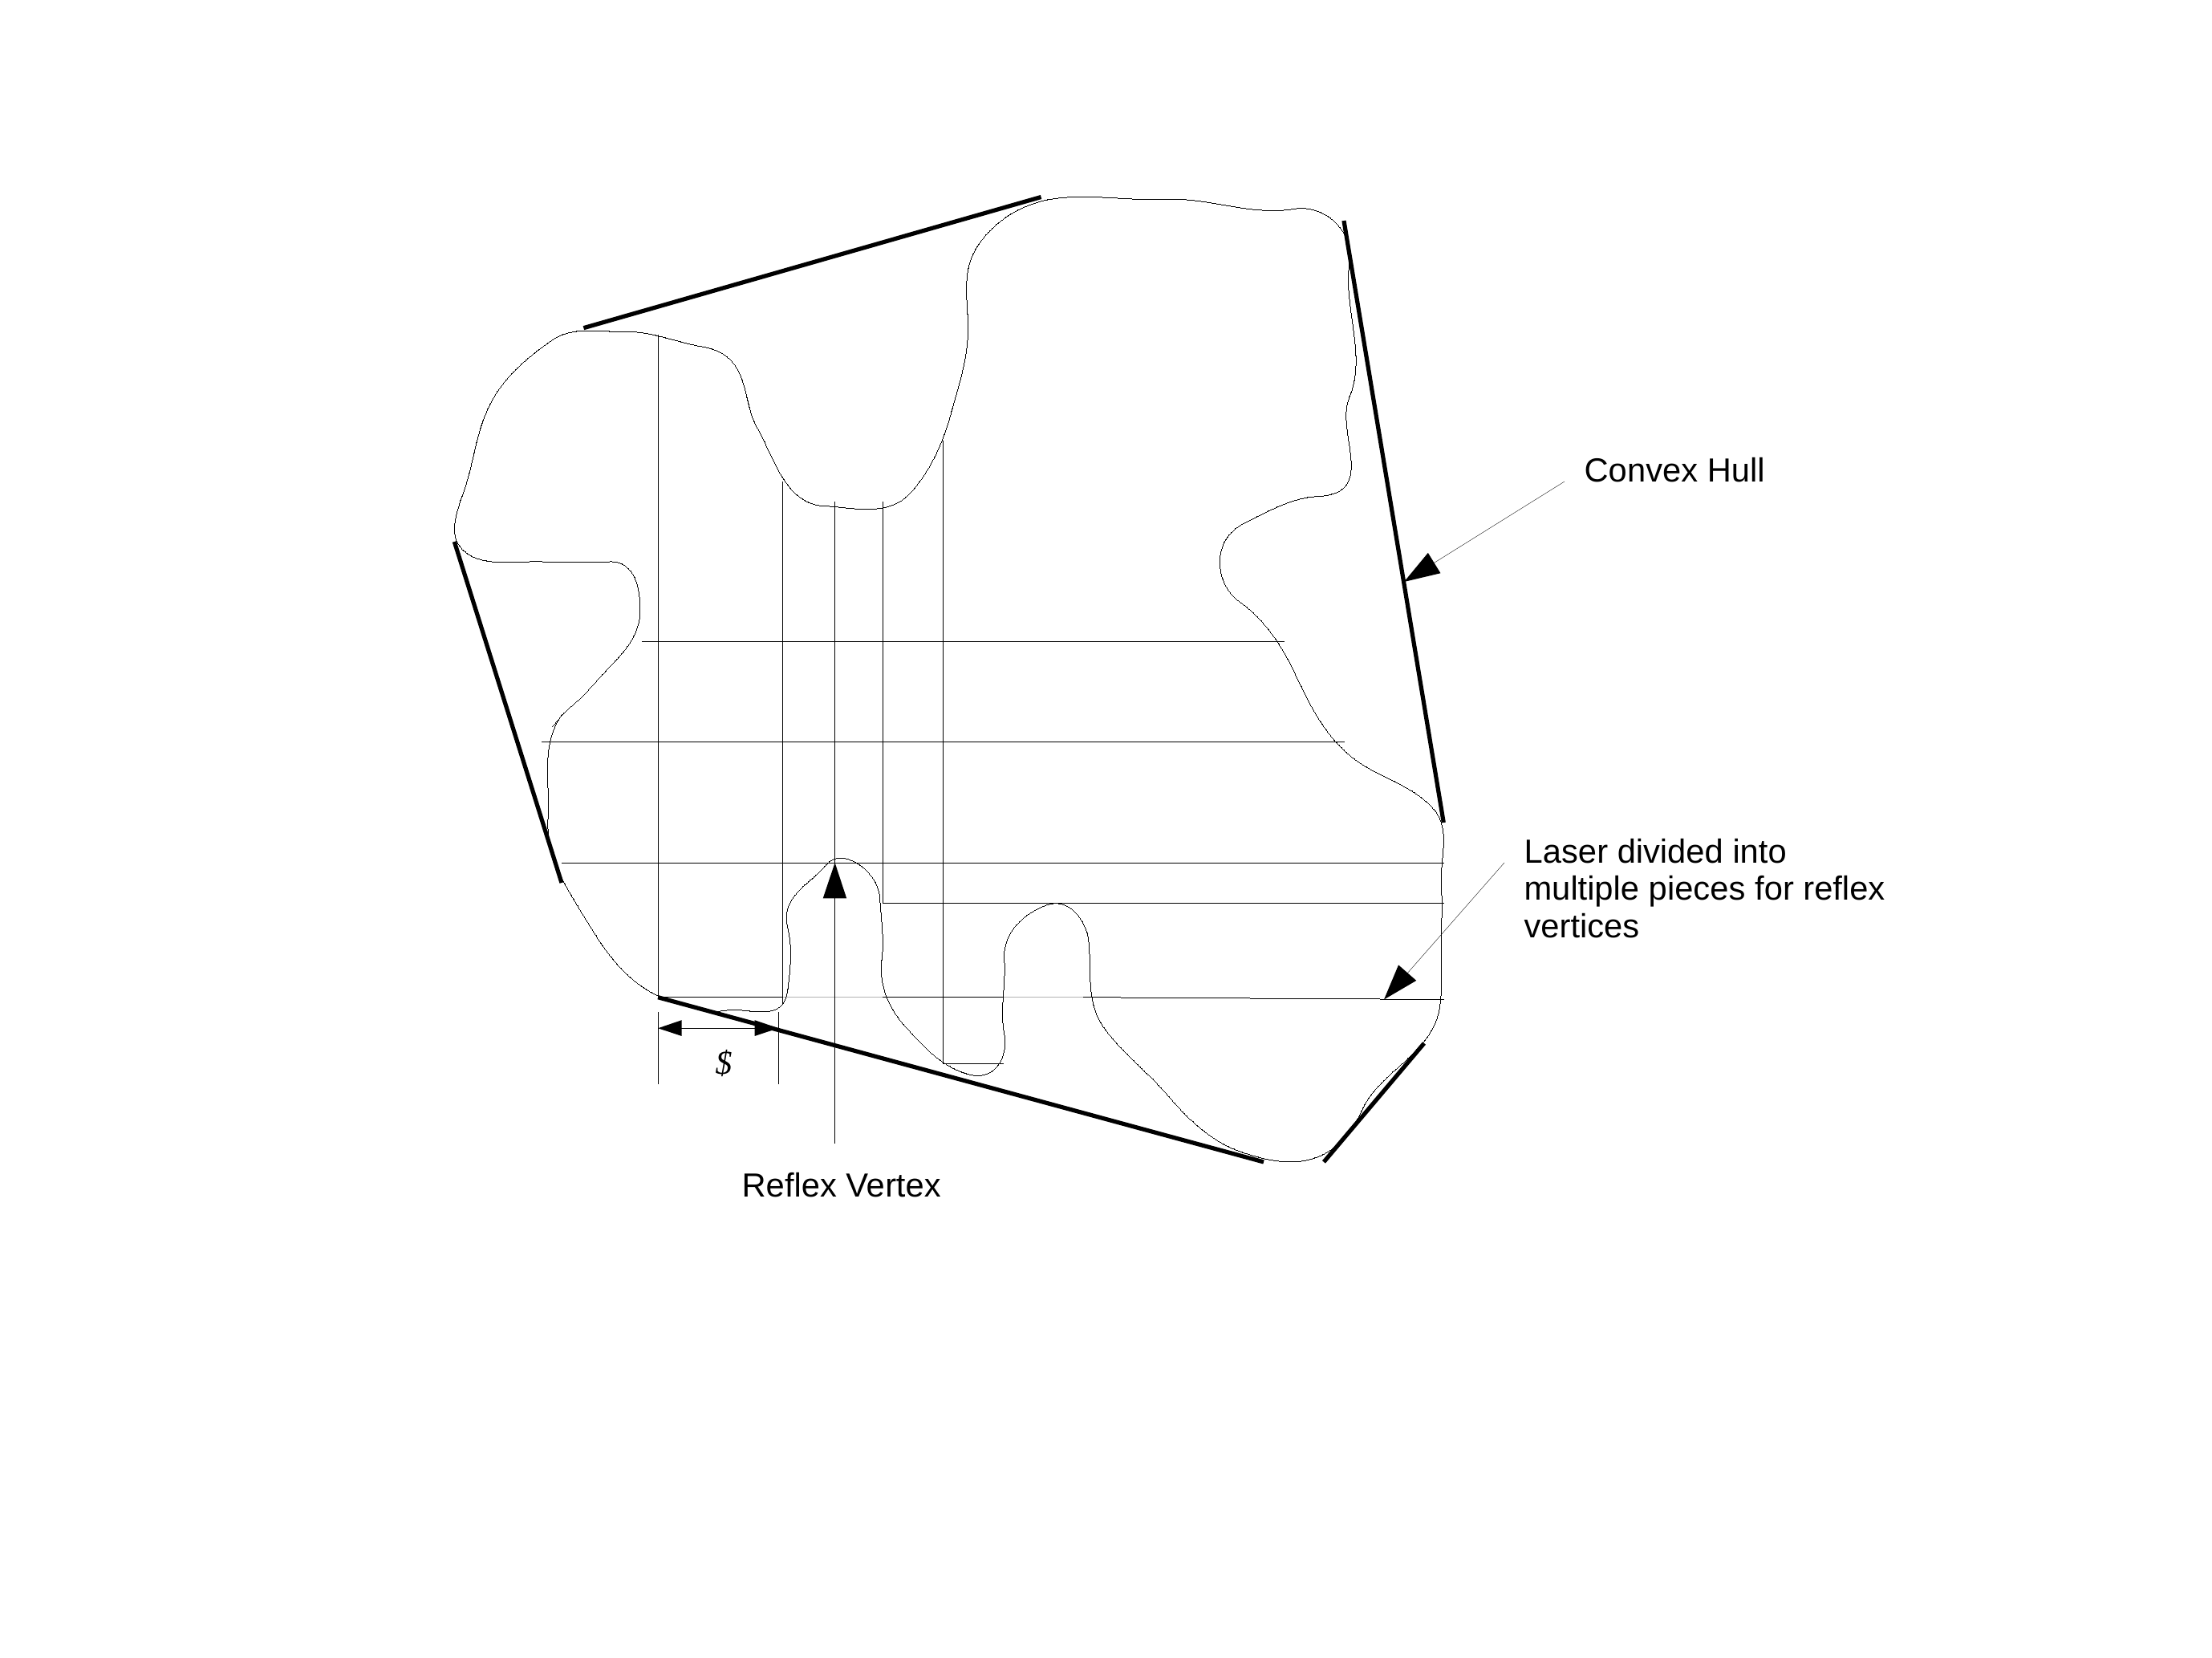}
	\caption{Minimize diameter of a partition}
	\label{fig:budget2}
\end{figure*}
	
\begin{proof}

	If there are $R$ reflex vertices in $P$, then cutting $\conv(P)$ with $\frac{K}{R}$ lasers will require $K$ lasers to touch the corresponding points in $P$ with $R$ reflex vertices. \\
	
	The optimum minimax diameter of $P$ cut by $K$ laser is greater than equal to the optimum minimax diameter of $\conv(P)$ cut by $K$ laser.
	
	Let $C_{X}(k)$ denotes the maximum diameter of a cut by k lasers in a convex polygon $X$ using algorithm described in Problem 3. \\
	
	$C_{X}^{*}(K)$ denotes the optimum maximum diameter of a cut by k lasers in a convex polygon $X$

	 \begin{equation}
	 \begin{aligned}
	 C_{\conv(P)}\Big(\frac{K}{R}\Big) &\leq 4\sqrt{2}\pi C_{\conv(P)}^{*}\Big(\frac{K}{R}\Big)  \\
	 &\leq 4\sqrt{2}\pi.O(R).C_{\conv(P)}^{*}(R) \\
	 &\leq O(R)C_{P}^{*}(R)
	  \end{aligned}
	  \end{equation}

\end{proof}

\subsection{Problem 5 : } Given a simple polygon $P$ with $r$ reflex vertices and an area budget $\delta$, find the smallest number of lasers such that each partition created by the cuts of lasers has area less than equal to $\delta$.

\subsubsection{Algorithm}
\begin{enumerate}
	\item Make a sequence of the reflex vertices (counter-clock wise along the polygon boundary from left most reflex vertex).
	\item Create a empty vertex list $L$.
	\item From each reflex vertex $v_{i}$ draw its angle bisector. Lets suppose the bisector hits at edge $v_{i}^{1}v_{i}^{2}$. then we add these 2 vertices $v_{i}^{1}$ and $v_{i}^{2}$ to vertex list $L$.
	\item When all the reflex vertex are exhausted, create a sequence of vertices(counter-clock wise order) added in list L. Note that, here total number of vertices in $L$ can be at most $3r$.
	\item Now, choose 3 vertices from $L$ which are equally-spaced in original polygon $P$. Compute geodesic triangle using these vertices.
	\item Create a geodesic triangulation tree as described in \cite{suri} by Hershberger and Suri.
	\item This will create a tree of degree 3 and each node will be a geodesic triangle.
	\item We will then divide each geodesic triangle into ordinary triangles using steiner points as described in \cite{suri}. Hence, it creates a bounded degree hierarchy.
	\item Merge the triangle leaves with their parents till the summation of area of the merged parent+children region $\leq \delta$
%	8) Once we get a triangulation after finishing step 7, we call merge subroutine. Here, we merge a set of adjacent triangles each has area less than $\delta$ in a pseudo-triangle such that if we merge $m$ such triangles, then before we add $m-th$ triangle the size of already merged $m-1$ triangles is less than $\delta$.
%	9) After step 8, there may be some triangle or pseudo-triangle left over which has size less than $\delta$, but not merged with others. In that case we can merge them with adjacent big triangle or merged pseudo-triangle  As there is a constant number of triangle, hence in O(1) time, we can get minimum number of merged regions.
	\item Once the merged region become greater than $\delta$, we can put O(1) lasers so that cuts created by lasers have area less than $\delta$.
	\item For bigger triangle $t$, we can put $\theta(\sqrt{\area(t)/\delta})$ lasers to cut it pieces such that each piece has an area less than $\delta$.
\end{enumerate}

\subsubsection{Approximation Bound:}	
\begin{theorem}
	Problem 5 can be solved by a  polynomial time $\log(r)$ approximation algorithm.
\end{theorem}

\begin{proof}
	Each region whose area is above the threshold delta will intersect a laser in OPT. Since each region is the union of one or more triangles of the Hershberger-Suri triangulation, every laser in OPT intersects O(log r) such regions.
	Consequently,  $|regions| = O(|OPT| \log r)$, which gives $|OPT| = \omega(|regions| / \log r)$, where $|regions|$ is the number of merged regions.  So, when we use $O(1)$ lasers for each such region, we create a $O(\log r)$ approximation. Also, for large triangle we are putting optimum number of lasers, hence the approximation bound holds.
\end{proof}

\section{Without Convex Piece Decomposition Restriction:}

\subsection{Problem 6:} Given a simple polygon with $r$ reflex vertex and an area budget $\delta$ we have a $O(\log r)$ approximation to minimize the number of laser where pieces can be non-convex.
\subsubsection{Algorithm}
Same as the algorithm for problem 5.

\subsubsection{Approximation Bound:}
\begin{theorem}
	Problem 5 can be solved by a  polynomial time $log(r)$ approximation algorithm.
\end{theorem}

\begin{proof}
	Even though, there is no restriction that each piece has to be convex, the lower bound of number of laser id still same as of problem 5, i.e. $|OPT| = \omega(|regions| / \log r)$. Hence by putting O(1) lasers per merged region and optimum number of lasers for large triangle, we will get a $O(\log r)$ approximation.
\end{proof}
